# Supplementary material for: Data-Driven Permissible Safe Control with Barrier Certificates
Source: arXiv:2405.00136 source file (2024-05-05)
Supplement: Supplementary file 1 [file 7_appendix.tex]

\section{Misc}

Probably not useful

\subsection{GP Bounding Adjustment}
\JS{This is more of an implementation detail.}
In Section .. , the proposed GP formulation takes the form 
$$
   x_{k+1}  = \Gm + \Gv.
$$
To facilitate better regression with GPs, we learn the change the current point $x_k$, or
$$
x_{k+1} = x_k + \Gm + \Gv.
$$
which is equivalent to setting a prior mean function that relies on $x$, i.e. $m_0(x) = x$. 
Therefore, given $x_k$ and bounds $[\lGm, \uGm]$, 
$$
x_{k+1} \in [x_k + \lGm, x_k + \uGm].
$$
Likewise, given an interval of possible inputs, $[x^L_k, x^U_k]$, the range of possible outputs is $[x^L_{k+1}, x^U_{k+1}]$ where \JS{incorrect notation below for mean bounds over interval}
$$
x^L_{k+1} = x^L_k + \lGm,~~x^U_{k+1} = x^U_k + \uGm
$$

\subsection{Polynomial Kernel}
The polynomial kernel is

\begin{align}
\kernel(x_1,x_2) &= \var(x_1'x_2 + c)^d
\end{align}

So the posterior mean is (zero prior)
$$
\mean(x) = \sum_{j=1}^m\var\alpha_j(x'x_j+c)^d
$$
and the posterior variance (conditioned on the dataset $D$) is 
$$
\std_\dataset^2(x) = \var(x'x+c)^d-\sum_{i=1}^\datasetsize \var(x'x_i+c)^d\sum_{j=1}^\datasetsize K^{-1}_{i,j}\var(x'x_j+c)^d
$$
where $\datasetsize=|\dataset|$ is the size of the training dataset.
In addition, the total variance is this posterior variance plus the noise variance:
$$
\std_{total}^2(x) = \var(x) + R
$$

\subsection{Exponential Kernel}

Bounds on GP:

$$\tilde{A}
+
\tilde{C}
+
\tilde{B} x^{T} \theta I x
-
\tilde{D}x
\geq \mu(x)
\geq 
A
+
C
+
B x^{T} \theta I x
- Dx
$$

\subsection{Random Tools}
https://en.wikipedia.org/wiki/Pad%C3%A9_approximant

Upper bound based on :

https://stackoverflow.com/questions/42732225/fast-integer-sqrt-upper-bound-approximation

\section{Sum-of-Squares Barrier}

Using piecewise barrier now

The synthesis of a stochastic barrier certificate can be formulated as a nonlinear optimization problem, which can be solved efficiently using convex optimization. We define an SOS polynomial as

\begin{definition}[SOS Polynomial]
    \label{def:sosp1}
    A multivariate polynomial $\lambda(x)$ is  a Sum-Of-Squares (SOS) for $x \in \mathbb{R}^{n}$ if there exists some polynomials $\lambda_{i}$, $i = 1, \ldots, r$, for some ${r \in \naturals}$, such that
    $\lambda(x) = \sum_{i=1}^{r} \lambda_{i}^{2}(x) \geq 0.$
    % If $\lambda(x)$ is an SOS, then $\lambda(x) \geq 0$ for all $x \in \mathbb{R}^{n}$. 
    The set of all SOS polynomials is denoted by $\Lambda$.
\end{definition}

Consider a basic closed semi-algebraic set $X =\set{x \in \reals^n \mid h_i(x) \geq 0  \;\; \forall i \in \set{1, \ldots, l}}$, which is defined as the intersection of $l$ polynomial ($h_i(x)$) inequalities. 
\begin{proposition}[Putinar’s Certificate, \cite{Stengle1974}]
    \label{prop:sosp1}
    Polynomial $\gamma(x)$ is non-negative on $X$ if,   for some $ \lambda_{0}(x), \lambda_{i}(x) \in \Lambda$,
    % \begin{equation*}
        $\gamma (x) = \lambda_0(x) + \sum_{i=1}^{l} \lambda_{i}(x) h_{i}(x).$
    % \end{equation*}
\end{proposition}

Using these properties, Theorem \ref{th:sosp_gpbarrier} shows how the Probabilistic N-Invariant sets can be obtained for a GP model using a barrier approach. In particular, the theorem shows how to formulate Conditions -- as SOS constraints. 

\RM{Combine theorem 1 and 2 into 1...}

% \begin{proof}
% It suffices to show that if $B$ satisfies Constraints \eqref{constraint1}-\eqref{constraint4}, then Conditions \eqref{Eq:Cond3}-\eqref{Eq:Cond5} are satisfied. 
% As Constraint \eqref{constraint1} guarantees that $B$ is a SOS polynomial, hence non-negative by definition, Condition \eqref{Eq:Cond3} holds. 
% By Corollary \ref{cor:sosp1} it holds that if Constraints \eqref{constraint2}-\eqref{constraint3} hold, then $B$ is respectively smaller that $\eta$ in $X_0$ and greater than $1$ in $X_u$. What is left to show is that Constraint \eqref{constraint4} guarantees the satisfaction of Condition \eqref{Eq:Cond5}. This can be done as follows. 
% For every region $q \in Q$,
% the expectation term in Condition \eqref{Eq:Cond5} can be expressed as $E[B(y + v) \mid x]$, where $y$ is bounded by under-approximation $\low{f}_q(x)$ and over-approximation $\up{f}_q(x)$ of $\NN(x)$ in System \eqref{Eqn:SystemEqn}  for all $x \in q$.  Then by Corollary \ref{cor:sosp1}, Constraint \eqref{constraint4} is obtained for each $q$.  Note that $B(x)$ is a polynomial, so if $E[B(y + v) \mid x]$ is also a polynomial, the condition is a valid SOS constraint.  Given that $y + v$ is linear, $E[B(y + v) \mid x]$ is a sum of monomials in terms of $y$ and expectation moments $\mathbb{E}[v^{d}]$, where $d \geq 0$. Since, random variable $v$ has a normal distribution, $\mathbb{E}[v^{d}]$ is  constant.  Therefore, $E[B(y + v) \mid x]$ is a polynomial only in terms of (components of) $y$. 
% \end{proof}

\RM{Remove SOS formulation}

\begin{theorem}[Probabilistic N-Invariant Sets]
    \label{th:sosp_gpbarrier}
    Consider SOS polynomial function $B(x)$, and
    % sets
    % \begin{itemize}
    %     \item safe set $ X_\safe = \set{  x \in \reals^{n} : h_{\safe}(x) \geq 0}$, 
    %     \item initial set $ X_{\initial} = \set{  x \in \reals^{n} : h_{\initial}(x) \geq 0}$, 
    %     \item unsafe set $X_{\unsafe} = \reals^n \setminus X_\safe = \set{  x \in \reals^{n} : h_{{\unsafe}}(x) \geq 0}$, and
    %     \item partition region $X_q= \set{  x \in \reals^{n} : h_{{q}}(x) \geq 0 }$ for all $q \in Q$.
    % \end{itemize}
    safe set $ X_\safe = \set{  x \in \reals^{n} \mid h_{\safe}(x) \geq 0}$, 
    initial set $ X_{\initial} = \set{  x \in \reals^{n} \mid h_{\initial}(x) \geq 0}$, 
    unsafe set $X_{\unsafe} = \reals^n \setminus X_\safe = \set{  x \in \reals^{n} \mid h_{{\unsafe}}(x) \geq 0}$, and
    partition region $q= \set{  x \in \reals^{n} \mid h_{{q}}(x) \geq 0 }$ for all $q \in Q$.
    Let $\mathcal{L}_{\safe}(x)$, $\mathcal{L}_{\initial}(x)$ and $\mathcal{L}_{\unsafe}(x)$ be vectors of SOS polynomials with the same dimensions as $h_\safe$, $h_\initial$, and $h_\unsafe$, respectively. Likewise, let $\mathcal{L}_{q,x}(x)$  and $ \mathcal{L}_{q, m}(x)$ be vectors of SOS polynomials with the same dimension as $h_q$ and $\Gm$, respectively. Finally, let $\mathcal{L}_{q}(\std)$ be a $n$-dimensional vector of polynomials.
   Then, a stochastic barrier certificate $B(x)$ for System~\eqref{eq:system} with time horizon $N \in \naturals_{\geq 0}$ can be obtained by solving the following SOS optimization problem for $\eta,\beta \in [0,1]:$
    \begin{subequations}
    \begin{align}
        % \label{eq:OptimProb}
        &\min_{\beta,\eta} \quad \eta + \beta  N \qquad
         \text{subject to:} \nonumber \\
        & \hspace{0.5mm} B(x)\in \Lambda, \label{constraintGP1} \\
        \hspace{0.5mm} - &  B(x) - \mathcal{L}^{T}_{\initial}(x)h_{\initial}(x) + \eta \in \Lambda, \label{constraintGP2}  \\
        & \hspace{0.5mm} B(x) - \mathcal{L}^{T}_{\unsafe}(x)h_{\unsafe}(x) -1 \in \Lambda, \label{constraintGP3} \\
        % \begin{split}
                 & \hspace{0.5mm} -E[B( y + {v}) \mid x]  + B(x) /\alpha + \beta -  \mathcal{L}^{T}_{q,x}(x)h_{q}(x) - \nonumber \\
                 & \hspace{7.5mm} \mathcal{L}^{T}_{q, m}(x)
                 \left (
                 (\lGm - m)\odot(m - \uGm)
                 \right ) - 
                 \\
                & \hspace{7.5mm}
                 \mathcal{L}^{T}_{q}(\std)
                  \left (
                 (\up{\std}_q - \std)\odot(\std - \low{\std}_q)
                 \right ) 
                 \in \Lambda \hspace{10mm}   \label{constraintGP4}      
        % \end{split}
        \forall q \in Q
    \end{align}
    \end{subequations}
    where $\odot$ denotes the element-wise Schur product. This
    guarantees safety probability
    $P_\safe(X_\safe,X_0,N ) \geq 1 - (\eta + \beta N)$. 
\end{theorem}

\section{Active Learning}

Active learning is an intelligent procedure to collect additional data to satisfy an objective. 
Our objective is to increase the size of the control invariant set while remaining safe. 

Our active learning procedure uses a greedy action-selection criterion on the discrete states $Q$, and the continuous space $X$. 

This criterion is the maximum variance according to the posterior GP given the current dataset $D_k$ where $k$ denotes the current step in the online setting. 
Recall for a given point $(x,u)$, the posterior variance is $\var(x,u)$ and for discrete state $q=\{[x_L, x_U], [u_L,u_U]\}$ the variance for all points therein is upper-bounded by $\up\var(q)$.

\subsection{Discrete Control Selection}
Given the current state $x_k$, the most valuable control interval according to $\up\var(q)$. 

The motivation behind choosing the interval first is that 1) the interval has already been deemed safe, so we know the system will remain safe with high probability for any action selected from the interval, and 2) choosing the interval where there is the highest uncertainty $\up\var(q)$ means the most information stands be be collected.

\subsection{Continuous Control Selection}
After the best control interval is chosen, it remains to find the value of the continuous control $u_k$ in the interval that maximizes $\var(x_k,u_k)$. 
For the squared-exponential kernel, this can be done by employing bounds. 
Otherwise, a suboptimal choice of $u_k$ can be found via sampling the GP posterior.
This can be done cheap and fast, online. 

\subsection{Barrier Updates}
\JS{Current setup with barriers only lets us reason about the control. GPs can be used to reason about states we want to reach from $x_k$}
Once a control input is selected and executed, the resulting datapoint $(x_k, u_k, x_{k+1})$ can be used to update the GP regression, and in turn update the CBFs and control invariant set. 

As we have already identified some control invariant sets, we can focus on finding improvements in other non-safe sets. 
Let $Q^?$ be the set of possibly control invariant sets. 
Since we draw the control from interval $[u]$, we can try updating all states with $[u]\in q$. 

There are two options for updating the barrier:
\begin{itemize}
    \item Re-evaluate the barrier polynomial to get new values of $\beta$, 
    \item Recompute the barrier entirely
\end{itemize}
We provide a brief comparison of these two approaches in the case studies.

\subsubsection{No Safe Intervals}
What happens if, after executing a safe action $u_k$, the system enters a region $q$ that contains no control intervals that are safe with at least probability $p^*$? 
Can we reason \emph{a prior} about states where we can return %to $\ControlSafeSet$ in one step if we end up in them? 
Or are these actually not a concern?

\newpage

\subsection{PWCB}

\RM{Still think about this...}

\begin{theorem}[Piecewise Barrier with Partitioned Control]
Assume a piecewise function $B_i(x)$ over state partition $X_s = \cup_{i=1}^I X_i$, $x \in X_i $, 
control partition $U = \cup_{k=1}^K U_k$, $u \in U_k$, 
and stochastic process $\px' = f(x, u, v) $.
%, and time horizon $H\in \mathbb{N}$.
%Consider a piece-wise barrier $B_i(x)$ over the $i^{th}$ partition in set $X_s = \{X_1, \ldots, X_k \}$. 
% Then, $B(x) = \cup_{i=1}^K B_i(x)$ 
% is a piecewise stochastic barrier function if $\phantom{.} \forall i,j = \{1,\ldots, K\}$ $\exists \beta_j: X_j \to \mathbb{R}$ and $\exists \eta\geq 0$ such that the following conditions hold
\begin{subequations} 
    \begin{align}
        & B_{j}(x)\geq 0   &&  \hspace{-15mm} \forall j
        %\label{Eq:Cond3}
        \\ 
        & B_{j}(x)\leq \eta  && \hspace{-15mm} \forall j : X_j \cap X_0, \neq \emptyset
        \\
        & \indicator{B(x)} = 1  && \hspace{-15mm}\forall j : X_j \cap X_u, \neq \emptyset\\
        & \sum_{i = 1}^K \expect[B_i(\px') \mid \px' \in X_i] \cdot p(\px' \in X_i) && \nonumber \\
        & \quad + \indicator{X_u}(\px') \cdot p(\px' \in X_\unsafe)   \leq  B_{j}(x) + \beta_{j} && \forall x \in X_j  
   %\label{Eq:Cond5}
    \end{align}
\end{subequations}
Minimization over the objective $\eta + N\cdot \max \beta_j$ guarantees safety probability $P_\safe(X_\safe,X_0, N) \geq 1 - (\eta + N\cdot \max \beta_j)$. 
\end{theorem}
