# Supplementary material for: Data-Driven Permissible Safe Control with Barrier Certificates
Source: arXiv:2405.00136 source file (2024-05-05)
Supplement: Supplementary file 2 [file 1_GP_bounding.tex]

\section{Misc}

Probably not useful

\subsection{GP Bounding Adjustment}
\JS{This is more of an implementation detail.}
In Section .. , the proposed GP formulation takes the form 
$$
   x_{k+1}  = \Gm + \Gv.
$$
To facilitate better regression with GPs, we learn the change the current point $x_k$, or
$$
x_{k+1} = x_k + \Gm + \Gv.
$$
which is equivalent to setting a prior mean function that relies on $x$, i.e. $m_0(x) = x$. 
Therefore, given $x_k$ and bounds $[\lGm, \uGm]$, 
$$
x_{k+1} \in [x_k + \lGm, x_k + \uGm].
$$
Likewise, given an interval of possible inputs, $[x^L_k, x^U_k]$, the range of possible outputs is $[x^L_{k+1}, x^U_{k+1}]$ where \JS{incorrect notation below for mean bounds over interval}
$$
x^L_{k+1} = x^L_k + \lGm,~~x^U_{k+1} = x^U_k + \uGm
$$

\subsection{Polynomial Kernel}
The polynomial kernel is

\begin{align}
\kernel(x_1,x_2) &= \var(x_1'x_2 + c)^d
\end{align}

So the posterior mean is (zero prior)
$$
\mean(x) = \sum_{j=1}^m\var\alpha_j(x'x_j+c)^d
$$
and the posterior variance (conditioned on the dataset $D$) is 
$$
\std_\dataset^2(x) = \var(x'x+c)^d-\sum_{i=1}^\datasetsize \var(x'x_i+c)^d\sum_{j=1}^\datasetsize K^{-1}_{i,j}\var(x'x_j+c)^d
$$
where $\datasetsize=|\dataset|$ is the size of the training dataset.
In addition, the total variance is this posterior variance plus the noise variance:
$$
\std_{total}^2(x) = \var(x) + R
$$

\subsection{Exponential Kernel}

Bounds on GP:

$$\tilde{A}
+
\tilde{C}
+
\tilde{B} x^{T} \theta I x
-
\tilde{D}x
\geq \mu(x)
\geq 
A
+
C
+
B x^{T} \theta I x
- Dx
$$

\subsection{Random Tools}
https://en.wikipedia.org/wiki/Pad%C3%A9_approximant

Upper bound based on :

https://stackoverflow.com/questions/42732225/fast-integer-sqrt-upper-bound-approximation
