# Supplementary material for: Data-Driven Permissible Safe Control with Barrier Certificates
Source: arXiv:2405.00136 source file (2024-05-05)
Supplement: Supplementary file 3 [file 2_BarrierSOS.tex]

\section{Sum-of-Squares Barrier}

Using piecewise barrier now

The synthesis of a stochastic barrier certificate can be formulated as a nonlinear optimization problem, which can be solved efficiently using convex optimization. We define an SOS polynomial as

\begin{definition}[SOS Polynomial]
    \label{def:sosp1}
    A multivariate polynomial $\lambda(x)$ is  a Sum-Of-Squares (SOS) for $x \in \mathbb{R}^{n}$ if there exists some polynomials $\lambda_{i}$, $i = 1, \ldots, r$, for some ${r \in \naturals}$, such that
    $\lambda(x) = \sum_{i=1}^{r} \lambda_{i}^{2}(x) \geq 0.$
    % If $\lambda(x)$ is an SOS, then $\lambda(x) \geq 0$ for all $x \in \mathbb{R}^{n}$. 
    The set of all SOS polynomials is denoted by $\Lambda$.
\end{definition}

Consider a basic closed semi-algebraic set $X =\set{x \in \reals^n \mid h_i(x) \geq 0  \;\; \forall i \in \set{1, \ldots, l}}$, which is defined as the intersection of $l$ polynomial ($h_i(x)$) inequalities. 
\begin{proposition}[Putinar’s Certificate, \cite{Stengle1974}]
    \label{prop:sosp1}
    Polynomial $\gamma(x)$ is non-negative on $X$ if,   for some $ \lambda_{0}(x), \lambda_{i}(x) \in \Lambda$,
    % \begin{equation*}
        $\gamma (x) = \lambda_0(x) + \sum_{i=1}^{l} \lambda_{i}(x) h_{i}(x).$
    % \end{equation*}
\end{proposition}

Using these properties, Theorem \ref{th:sosp_gpbarrier} shows how the Probabilistic N-Invariant sets can be obtained for a GP model using a barrier approach. In particular, the theorem shows how to formulate Conditions -- as SOS constraints. 

\RM{Combine theorem 1 and 2 into 1...}

% \begin{proof}
% It suffices to show that if $B$ satisfies Constraints \eqref{constraint1}-\eqref{constraint4}, then Conditions \eqref{Eq:Cond3}-\eqref{Eq:Cond5} are satisfied. 
% As Constraint \eqref{constraint1} guarantees that $B$ is a SOS polynomial, hence non-negative by definition, Condition \eqref{Eq:Cond3} holds. 
% By Corollary \ref{cor:sosp1} it holds that if Constraints \eqref{constraint2}-\eqref{constraint3} hold, then $B$ is respectively smaller that $\eta$ in $X_0$ and greater than $1$ in $X_u$. What is left to show is that Constraint \eqref{constraint4} guarantees the satisfaction of Condition \eqref{Eq:Cond5}. This can be done as follows. 
% For every region $q \in Q$,
% the expectation term in Condition \eqref{Eq:Cond5} can be expressed as $E[B(y + v) \mid x]$, where $y$ is bounded by under-approximation $\low{f}_q(x)$ and over-approximation $\up{f}_q(x)$ of $\NN(x)$ in System \eqref{Eqn:SystemEqn}  for all $x \in q$.  Then by Corollary \ref{cor:sosp1}, Constraint \eqref{constraint4} is obtained for each $q$.  Note that $B(x)$ is a polynomial, so if $E[B(y + v) \mid x]$ is also a polynomial, the condition is a valid SOS constraint.  Given that $y + v$ is linear, $E[B(y + v) \mid x]$ is a sum of monomials in terms of $y$ and expectation moments $\mathbb{E}[v^{d}]$, where $d \geq 0$. Since, random variable $v$ has a normal distribution, $\mathbb{E}[v^{d}]$ is  constant.  Therefore, $E[B(y + v) \mid x]$ is a polynomial only in terms of (components of) $y$. 
% \end{proof}

\RM{Remove SOS formulation}

\begin{theorem}[Probabilistic N-Invariant Sets]
    \label{th:sosp_gpbarrier}
    Consider SOS polynomial function $B(x)$, and
    % sets
    % \begin{itemize}
    %     \item safe set $ X_\safe = \set{  x \in \reals^{n} : h_{\safe}(x) \geq 0}$, 
    %     \item initial set $ X_{\initial} = \set{  x \in \reals^{n} : h_{\initial}(x) \geq 0}$, 
    %     \item unsafe set $X_{\unsafe} = \reals^n \setminus X_\safe = \set{  x \in \reals^{n} : h_{{\unsafe}}(x) \geq 0}$, and
    %     \item partition region $X_q= \set{  x \in \reals^{n} : h_{{q}}(x) \geq 0 }$ for all $q \in Q$.
    % \end{itemize}
    safe set $ X_\safe = \set{  x \in \reals^{n} \mid h_{\safe}(x) \geq 0}$, 
    initial set $ X_{\initial} = \set{  x \in \reals^{n} \mid h_{\initial}(x) \geq 0}$, 
    unsafe set $X_{\unsafe} = \reals^n \setminus X_\safe = \set{  x \in \reals^{n} \mid h_{{\unsafe}}(x) \geq 0}$, and
    partition region $q= \set{  x \in \reals^{n} \mid h_{{q}}(x) \geq 0 }$ for all $q \in Q$.
    Let $\mathcal{L}_{\safe}(x)$, $\mathcal{L}_{\initial}(x)$ and $\mathcal{L}_{\unsafe}(x)$ be vectors of SOS polynomials with the same dimensions as $h_\safe$, $h_\initial$, and $h_\unsafe$, respectively. Likewise, let $\mathcal{L}_{q,x}(x)$  and $ \mathcal{L}_{q, m}(x)$ be vectors of SOS polynomials with the same dimension as $h_q$ and $\Gm$, respectively. Finally, let $\mathcal{L}_{q}(\std)$ be a $n$-dimensional vector of polynomials.
   Then, a stochastic barrier certificate $B(x)$ for System~\eqref{eq:system} with time horizon $N \in \naturals_{\geq 0}$ can be obtained by solving the following SOS optimization problem for $\eta,\beta \in [0,1]:$
    \begin{subequations}
    \begin{align}
        % \label{eq:OptimProb}
        &\min_{\beta,\eta} \quad \eta + \beta  N \qquad
         \text{subject to:} \nonumber \\
        & \hspace{0.5mm} B(x)\in \Lambda, \label{constraintGP1} \\
        \hspace{0.5mm} - &  B(x) - \mathcal{L}^{T}_{\initial}(x)h_{\initial}(x) + \eta \in \Lambda, \label{constraintGP2}  \\
        & \hspace{0.5mm} B(x) - \mathcal{L}^{T}_{\unsafe}(x)h_{\unsafe}(x) -1 \in \Lambda, \label{constraintGP3} \\
        % \begin{split}
                 & \hspace{0.5mm} -E[B( y + {v}) \mid x]  + B(x) /\alpha + \beta -  \mathcal{L}^{T}_{q,x}(x)h_{q}(x) - \nonumber \\
                 & \hspace{7.5mm} \mathcal{L}^{T}_{q, m}(x)
                 \left (
                 (\lGm - m)\odot(m - \uGm)
                 \right ) - 
                 \\
                & \hspace{7.5mm}
                 \mathcal{L}^{T}_{q}(\std)
                  \left (
                 (\up{\std}_q - \std)\odot(\std - \low{\std}_q)
                 \right ) 
                 \in \Lambda \hspace{10mm}   \label{constraintGP4}      
        % \end{split}
        \forall q \in Q
    \end{align}
    \end{subequations}
    where $\odot$ denotes the element-wise Schur product. This
    guarantees safety probability
    $P_\safe(X_\safe,X_0,N ) \geq 1 - (\eta + \beta N)$. 
\end{theorem}
