# Supplementary material for: Data-Driven Permissible Safe Control with Barrier Certificates
Source: arXiv:2405.00136 source file (2024-05-05)
Supplement: Supplementary file 4 [file 3_ActiveLearning.tex]

\section{Active Learning}

Active learning is an intelligent procedure to collect additional data to satisfy an objective. 
Our objective is to increase the size of the control invariant set while remaining safe. 

Our active learning procedure uses a greedy action-selection criterion on the discrete states $Q$, and the continuous space $X$. 

This criterion is the maximum variance according to the posterior GP given the current dataset $D_k$ where $k$ denotes the current step in the online setting. 
Recall for a given point $(x,u)$, the posterior variance is $\var(x,u)$ and for discrete state $q=\{[x_L, x_U], [u_L,u_U]\}$ the variance for all points therein is upper-bounded by $\up\var(q)$.

\subsection{Discrete Control Selection}
Given the current state $x_k$, the most valuable control interval according to $\up\var(q)$. 

The motivation behind choosing the interval first is that 1) the interval has already been deemed safe, so we know the system will remain safe with high probability for any action selected from the interval, and 2) choosing the interval where there is the highest uncertainty $\up\var(q)$ means the most information stands be be collected.

\subsection{Continuous Control Selection}
After the best control interval is chosen, it remains to find the value of the continuous control $u_k$ in the interval that maximizes $\var(x_k,u_k)$. 
For the squared-exponential kernel, this can be done by employing bounds. 
Otherwise, a suboptimal choice of $u_k$ can be found via sampling the GP posterior.
This can be done cheap and fast, online. 

\subsection{Barrier Updates}
\JS{Current setup with barriers only lets us reason about the control. GPs can be used to reason about states we want to reach from $x_k$}
Once a control input is selected and executed, the resulting datapoint $(x_k, u_k, x_{k+1})$ can be used to update the GP regression, and in turn update the CBFs and control invariant set. 

As we have already identified some control invariant sets, we can focus on finding improvements in other non-safe sets. 
Let $Q^?$ be the set of possibly control invariant sets. 
Since we draw the control from interval $[u]$, we can try updating all states with $[u]\in q$. 

There are two options for updating the barrier:
\begin{itemize}
    \item Re-evaluate the barrier polynomial to get new values of $\beta$, 
    \item Recompute the barrier entirely
\end{itemize}
We provide a brief comparison of these two approaches in the case studies.

\subsubsection{No Safe Intervals}
What happens if, after executing a safe action $u_k$, the system enters a region $q$ that contains no control intervals that are safe with at least probability $p^*$? 
Can we reason \emph{a prior} about states where we can return %to $\ControlSafeSet$ in one step if we end up in them? 
Or are these actually not a concern?
