# Supplementary material for: Data-Driven Permissible Safe Control with Barrier Certificates
Source: arXiv:2405.00136 source file (2024-05-05)
Supplement: Supplementary file 5 [file 4_Derivations.tex]

\subsection{PWCB}

\RM{Still think about this...}

\begin{theorem}[Piecewise Barrier with Partitioned Control]
Assume a piecewise function $B_i(x)$ over state partition $X_s = \cup_{i=1}^I X_i$, $x \in X_i $, 
control partition $U = \cup_{k=1}^K U_k$, $u \in U_k$, 
and stochastic process $\px' = f(x, u, v) $.
%, and time horizon $H\in \mathbb{N}$.
%Consider a piece-wise barrier $B_i(x)$ over the $i^{th}$ partition in set $X_s = \{X_1, \ldots, X_k \}$. 
% Then, $B(x) = \cup_{i=1}^K B_i(x)$ 
% is a piecewise stochastic barrier function if $\phantom{.} \forall i,j = \{1,\ldots, K\}$ $\exists \beta_j: X_j \to \mathbb{R}$ and $\exists \eta\geq 0$ such that the following conditions hold
\begin{subequations} 
    \begin{align}
        & B_{j}(x)\geq 0   &&  \hspace{-15mm} \forall j
        %\label{Eq:Cond3}
        \\ 
        & B_{j}(x)\leq \eta  && \hspace{-15mm} \forall j : X_j \cap X_0, \neq \emptyset
        \\
        & \indicator{B(x)} = 1  && \hspace{-15mm}\forall j : X_j \cap X_u, \neq \emptyset\\
        & \sum_{i = 1}^K \expect[B_i(\px') \mid \px' \in X_i] \cdot p(\px' \in X_i) && \nonumber \\
        & \quad + \indicator{X_u}(\px') \cdot p(\px' \in X_\unsafe)   \leq  B_{j}(x) + \beta_{j} && \forall x \in X_j  
   %\label{Eq:Cond5}
    \end{align}
\end{subequations}
Minimization over the objective $\eta + N\cdot \max \beta_j$ guarantees safety probability $P_\safe(X_\safe,X_0, N) \geq 1 - (\eta + N\cdot \max \beta_j)$. 
\end{theorem}
